# Supplementary material for: SeedVR: Seeding Infinity in Diffusion Transformer Towards Generic Video Restoration
Source: arXiv:2501.01320 source file (2025-03-22)
Supplement: Supplementary file 1 [file X_suppl.tex]

\clearpage
\setcounter{page}{1}

\setboolean{putfigfirst}{true}
\ifthenelse{\boolean{putfigfirst}}{
\twocolumn[{%
\renewcommand\twocolumn[1][]{#1}%
\maketitlesupplementary\thispagestyle{empty}
\begin{center}
\refstepcounter{subfigure}\label{fig:netblock:a}
\refstepcounter{subfigure}\label{fig:netblock:b}
\includegraphics[width=\linewidth]{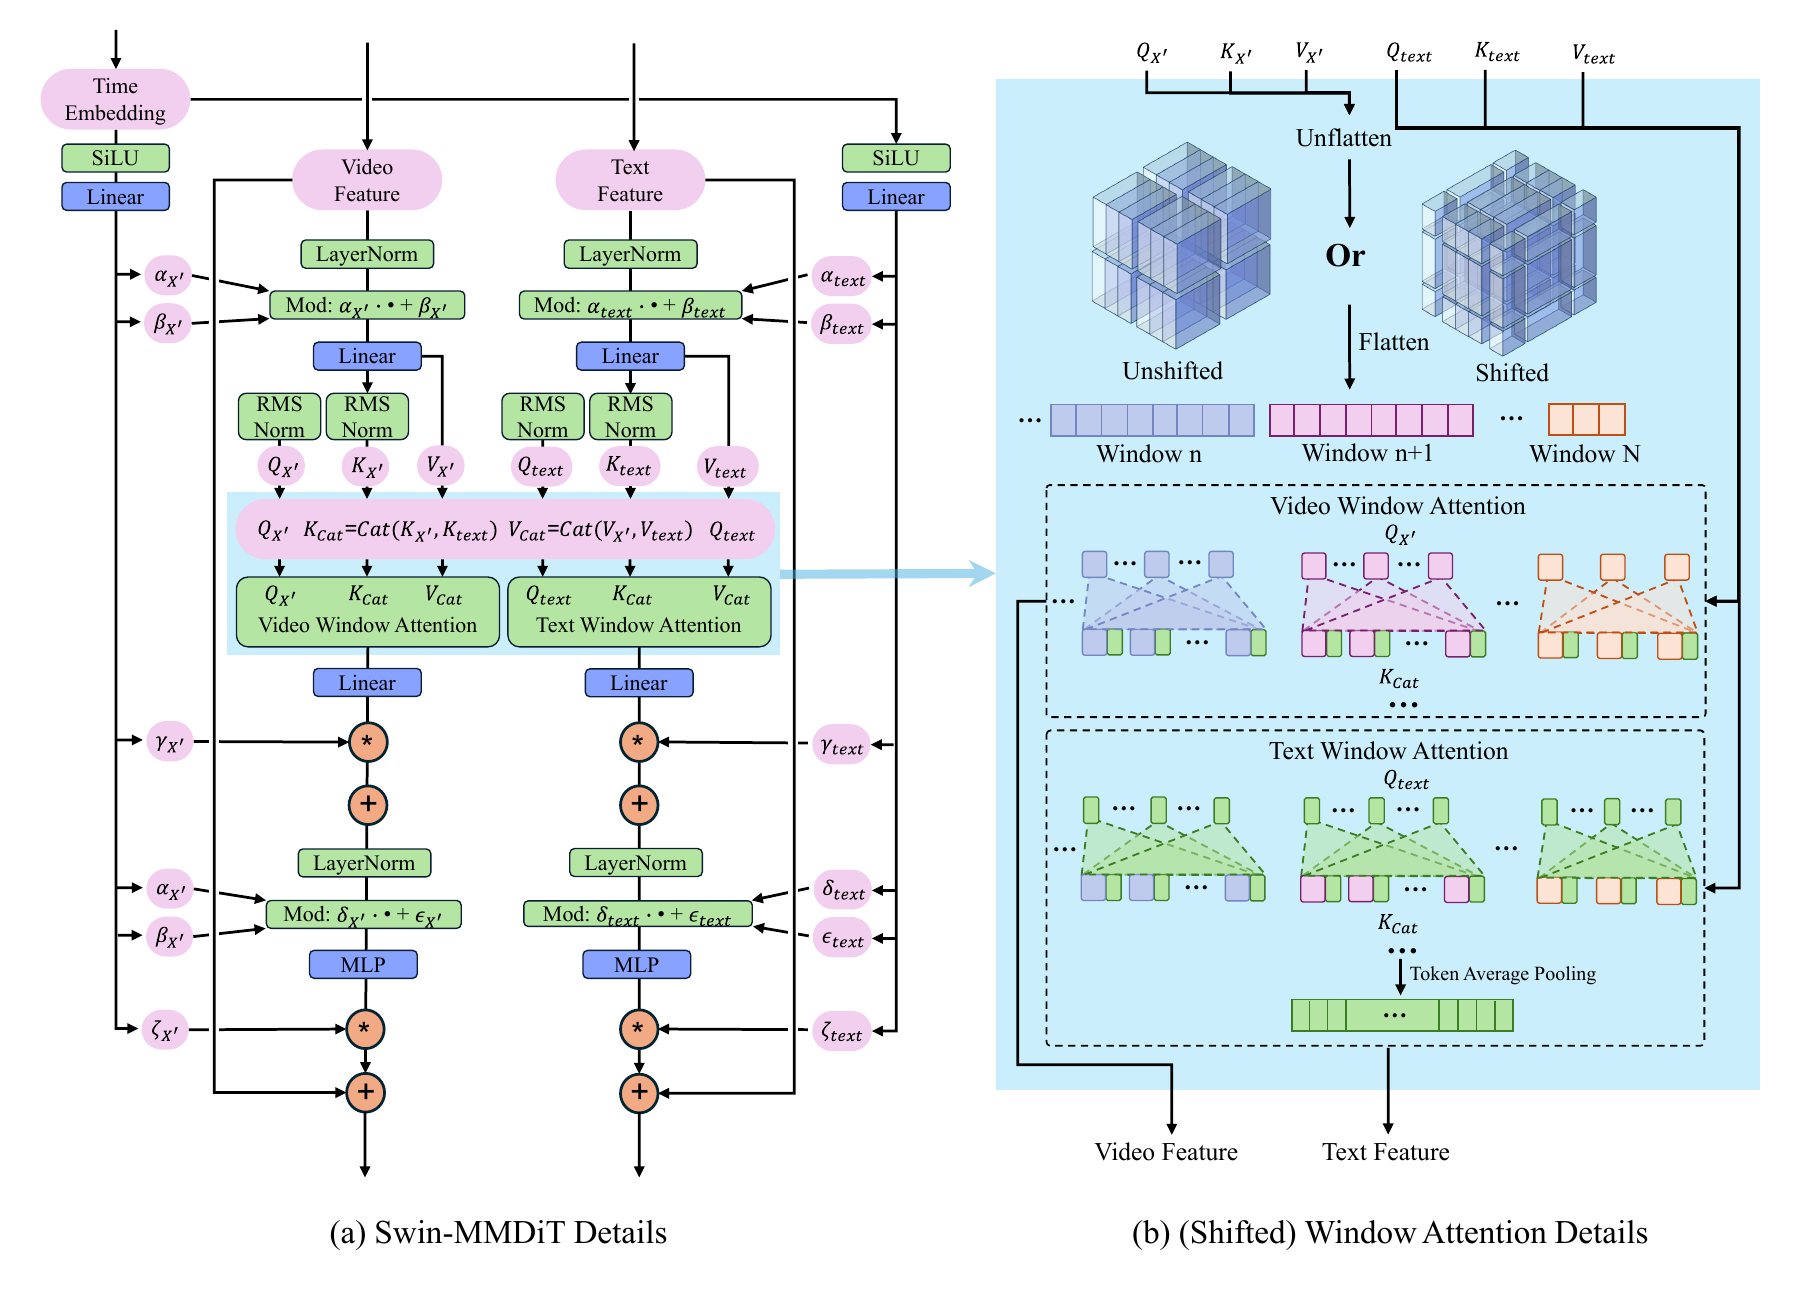}
\vspace{-7.5mm}
\captionof{figure}{Detailed architecture of Swin-MMDiT and the illustration of shifted window mechanism inside Swin-MMDiT. By introducing the proposed shifted window mechanism into the transformer block, our approach is capable of overcoming the resolution constraint of vanilla attention. We further adopt large attention windows around the center and variable-sized windows near the boundary, enabling long-range dependency capturing given inputs of any length and size.}
\vspace{0.5mm}
\label{fig:netblock}
\end{center}%
}]
}

\section{Video Demos}
\label{sec:demo}
We have added some video demos in the supplementary material for visualization.
For more video demos generated by our SeedVR, please refer to the project page: \href{https://iceclear.github.io/projects/seedvr/}{\texttt{\footnotesize{https://iceclear.github.io/projects/seedvr/}}} for details.

In the video demo, we mainly compare SeedVR with two state-of-the-art VR approaches~\cite{yang2023mgldvsr,he2024venhancer} due to the space limit.
Specifically, MGLD-VSR~\cite{yang2023mgldvsr} achieves high metric performance compared with other existing approaches in Table~\ref{tab:comparison}.
And VEnhancer~\cite{he2024venhancer} demonstrates superior enhancement performance compared with other existing baselines on AIGC videos. We adopt its latest checkpoint, i.e., venhancer\_v2.pth for comparison.
As shown in the demo, our SeedVR outperforms these two methods by a large margin on real-world videos.

\section{Detailed Architecture of Swin-MMDiT}
\label{sec:block}
As mentioned in Sec.~\ref{subsec:swin}, our Swin-MMDiT enhances the vanilla MMDiT~\cite{esser2024scaling} via introducing a shifted window mechanism.
Here, we further illustrate the detailed architecture in Figure~\ref{fig:netblock:a} as well as the window attention mechanism in Figure~\ref{fig:netblock:b}. 

Our design follows the principle of partitioning the vanilla full attention into window attention to overcome the resolution constraints.
Hence, we apply two window attentions for video and text features, respectively.

For video features, we adopt shifted large window, \ie $5 \times 64 \times 64$ to achieve long-range dependencies and introduce additional \textit{key} and \textit{value} from text features for text guidance.
To keep the flexibility for arbitrary resolutions, these text features interact with each video window feature.
And a 3D rotary position embedding~\cite{su2024roformer} is further adopted as a relative positional embedding in each window.
Such a flexible position embedding makes the model aware of varying-sized windows, bypassing the need to adjust the input resolution to be multiples of the window size.

For text features, directly making attention with the whole video features will bring the resolution constraint.
Instead, we assume the windows from the same video share the same text.
Thus, the text features are first repeated to interact with each window.
Then, the repeated features are combined via average pooling to maintain the same sequence length.

With a careful design of the window mechanism inside the Swin-MMDiT, our SeedVR is capable of handling any video input effectively and efficiently.
